# Supplementary material for: Effect of device design on charge offset drift in Si/SiO$_2$ single electron devices
Source: arXiv:1807.04342 source file (2018-07-11)
Supplement: Supplementary file 1 [file Supplement0709.pdf]

Supporting Information

# Effect of device design on charge offset drift in Si/$SiO_2$ single electron devices

Binhui Hu

Joint Quantum Institute, University of Maryland, College Park, Maryland 20742, USA

Erick D. Ochoa, Daniel Sanchez, and Justin K. Perron

California State University-San Marcos, San Marcos, CA 92069, USA

Neil M. Zimmerman and M. D. Stewart, Jr.

National Institute of Standards and Technology, Gaithersburg, MD, 20899, USA

This file includes:

S1. Equivalent circuit model to calculate the charge offset drift $Q_0(t)$ as a function of the defect charge variation $\Delta Q_d(t)$.

S2. FastCap simulation to quantitatively investigate the reduction of the charge offset drift before and after adding the top gate.

S3. Additional charge offset drift data (figures) from device 5.4-23U and device 4.7-33U, not presented in the main text.

## S1: Equivalent circuit model

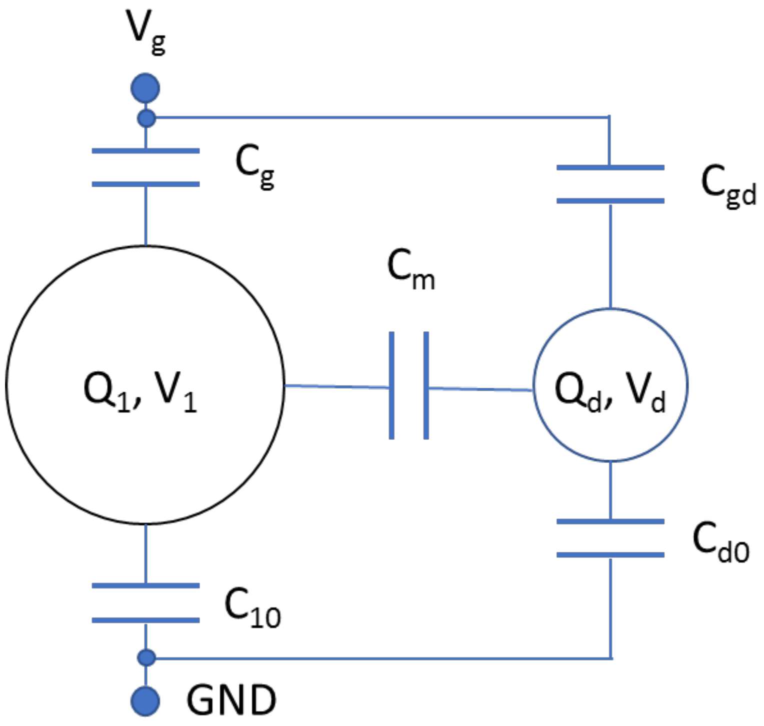


Figure S1. Equivalent circuit used to calculate the charge offset drift $Q_0(t)$ as a function of the defect charge variation $\Delta Q_d$, where one effective defect, $Q_d$, is coupled to the quantum dot, $Q_1$. $V_g$ is the sweeping gate voltage, which can be LEG, LCP, LLP, LIP, etc. The total capacitance for the quantum dot is $C_1=C_g+C_m+C_{10}$, and the total capacitance for the defect is $C_d=C_{gd}+C_m+C_{d0}$. $C_{10}$ ($C_{d0}$) includes the capacitance from the quantum dot (defect) to other no sweeping gate, source and drain leads. In case there is a top gate, $C_{10}$ ($C_{d0}$) includes the capacitance from the quantum dot (defect) to the top gate.

Consider a simplified case where one effective defect, $Q_d$, is coupled to the quantum dot, $Q_1$, in Fig. S1. Here we assume that the charge offset drift $Q_0(t)$ is only caused by the defect charge variation $\Delta Q_d(t)$ and all the capacitances are constant. Certainly defect charge motion can also cause $Q_0(t)$, but an infinitesimal motion can be modeled as an infinitesimal change of

the defect charge while keeping the capacitances constant. Our focus is to calculate the charge offset drift $Q_0$(t) as a function of the defect charge variation $\Delta Q_d$(t), and how adding a top gate can reduce such dependence.

We define $Q_0(t)$ as

$$Q_0(t) = -e\Delta V_g/(e/C_g) \tag{1}$$

Where $\Delta V_g$ is the voltage necessary to keep $Q_1$ and $V_1$ constant while the defect charge $Q_d$ changes by $\Delta Q_d$.

To keep $Q_1$ and $V_1$ the same,

$$C_g\Delta V_g = -C_m\Delta V_d \ . \tag{2}$$

$Q_0(t)$ arises because of the defect charge variation $\Delta Q_d$, which is

$$\Delta Q_d = C_m\Delta V_d + C_{d0}\Delta V_d + C_{gd}(\Delta V_d - \Delta V_g). \tag{3}$$

From Equations 1-3, we have

$$Q_0(t) = \Delta Q_d(t)/(C_d/C_m + C_{gd}/C_g), \tag{4}$$

where the total capacitance of the defect $C_d = C_{gd} + C_m + C_{d0}$.

For defects away from the gate, so that $C_{gd} \ll C_g$ , and $C_d/C_m \gg C_{gd}/C_g$,

$$Q_0(t) \approx (C_m/C_d)\Delta Q_d(t), \tag{5}$$

which doesn’t depend on which gate is used to measure the charge offset drift and the total capacitance of the quantum dot.

## S2: FastCap simulation

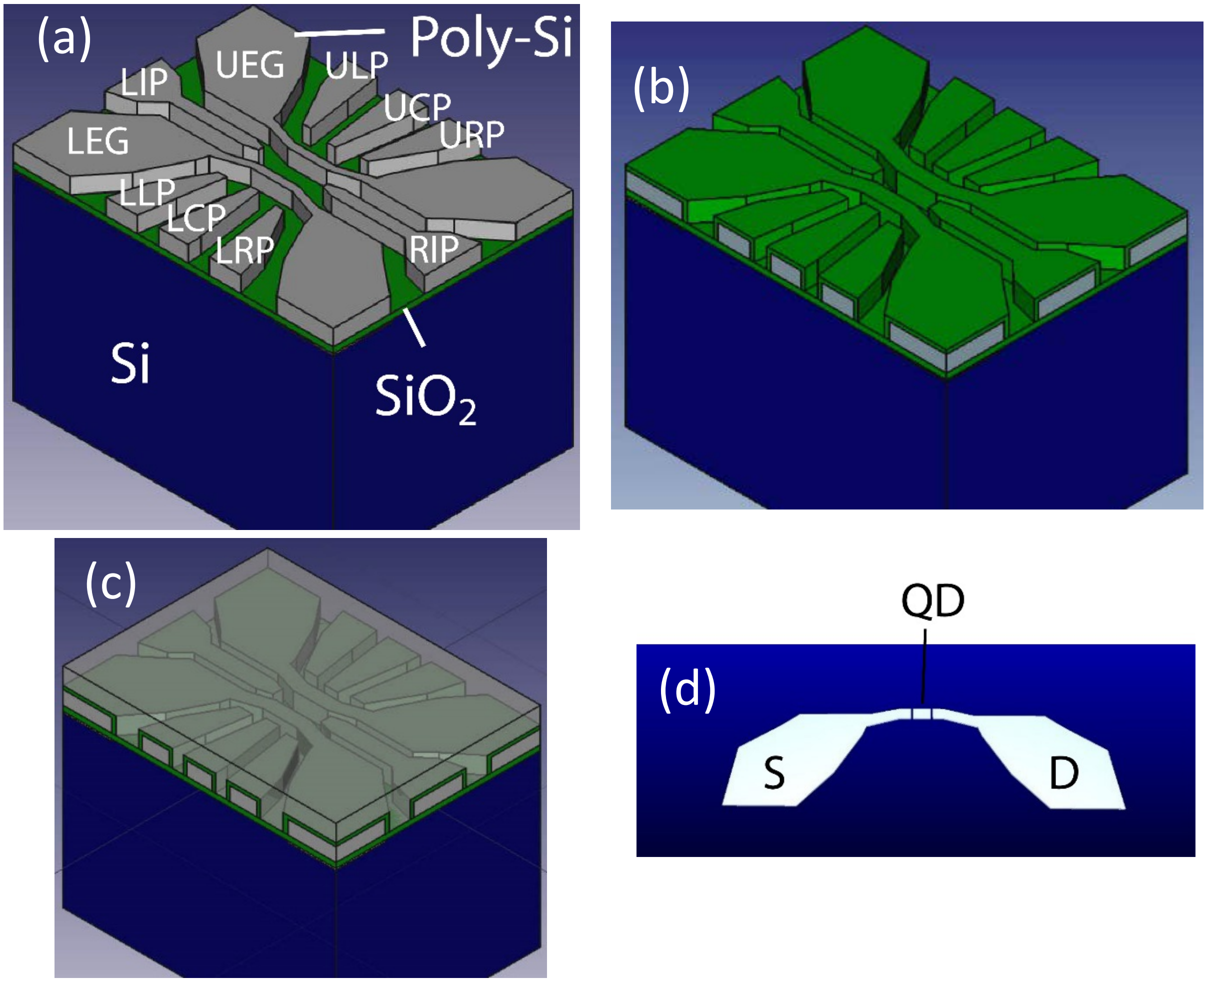


Figure S2. Three types of devices are simulated using FastCap. (a) a SED with no top gate or isolation oxide (”bare”). (b) a SED with 20 nm isolation oxide but no top gate (”oxide”). (c) a SED with 20 nm isolation oxide and a top gate (”TG”). (d) The quantum dot is located underneath LEG and at the $SiO_2$/Si interface, and modeled as a 40 nm x 80 nm x 10 nm metallic rectangular prism. It also has 10 nm gaps to the source and drain leads.

We have simulated three different types of devices using FastCap as shown in Fig. S2: a SED with no top gate or isolation oxide, called “bare”; a SED with 20 nm isolation oxide but no top gate, called “oxide”; and a SED with 20 nm isolation oxide and a top gate, called “TG”. The

gate oxide is 30 nm thick with the upper surface at z=0 and the $SiO_2$/Si interface at z=-30 nm. As a proof of concept, the quantum dot is modeled as a 40 nm x 80 nm x 10 nm metallic rectangular prism, located directly underneath LEG and at the $SiO_2$/Si interface. It also has 10 nm gaps to the source and drain leads. Capacitances to the quantum dot are shown in Table S1. For all FastCap simulations here, the tolerance is set at 1%. In all three cases, the total capacitance of the quantum dot doesn't change much from 40 aF which yields a 4 meV charging energy. Since measured quantum dots have a charging energy about 5 meV, their size should be quite similar, even though they are not necessarily intentional quantum dots.

| | "bare" | "oxide" | "TG" |
|---|---|---|---|
| Total | 40.4 | 41.0 | 41.8 |
| S, D | 13.0 | 11.6 | 10.9 |
| LEG | 6.6 | 7.6 | 5.2 |
| UEG | 2.7 | 2.8 | 1.3 |
| LIP, RIP | 0.5 | 0.5 | 0.25 |
| LCP | 1.6 | 1.9 | 0.74 |
| LLP, LRP | 0.65 | 0.73 | 0.31 |
| Top | | | 8.6 |

Talble S1. Capacitances from gates, S and D to the quantum dot in aF as derived from the Fastcap simulations for three different types of devices (1% tolerance).

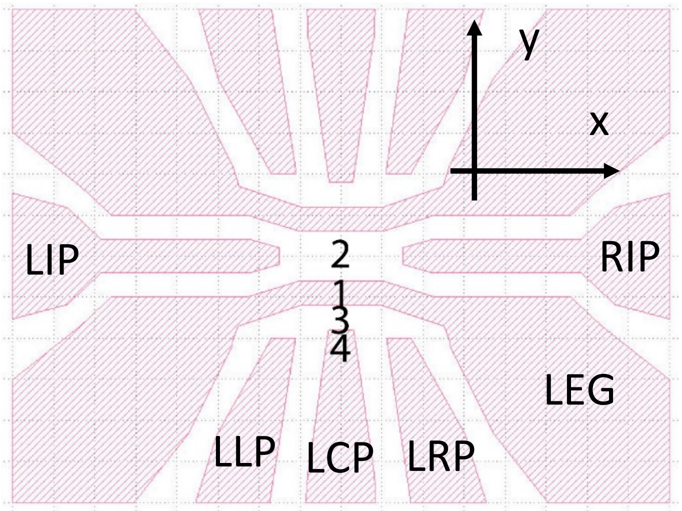


Figure S3. The defect is modeled as a 10 nm diameter metallic sphere. Four different lateral locations are calculated. Location 1: (0,-90 nm) directly underneath LEG; location 2: (0, 0) at the center; location 3: (0,-150 nm) and location 4: (0,-180 nm).

The defect is modeled as a 10 nm diameter metallic sphere. Four different lateral locations are simulated: location 1: (0,-90 nm) directly underneath LEG; location 2: (0, 0) at the center; location 3: (0,-150 nm) and location 4: (0,-180 nm). Since “bare” and “oxide” devices are quite similar (Table S1), we only compare the results between “bare” and “TG” devices. When the defect is located at the center of the gate oxide (z=-15 nm), the results are shown in Table S2 for “bare” and Table S3 for ”TG” devices.

(a) Location 1:

| Gate | $C_d$ | $C_m$ | $C_{gd}$ | $C_g$ | $A=C_m/C_d$ | $B=1/(C_d/C_m+C_{gd}/C_g)$ | \|A-B\|/B |
|---|---|---|---|---|---|---|---|
| LEG | 2.64 | 1.29 | 0.420 | 6.83 | 0.489 | 0.458 | 0.063* |
| LCP | 2.64 | 1.29 | 0.031 | 1.69 | 0.489 | 0.487 | 0.004 |
| LLP | 2.64 | 1.29 | 0.024 | 0.66 | 0.489 | 0.487 | 0.004 |
| LIP | 2.64 | 1.29 | 0.071 | 0.53 | 0.489 | 0.487 | 0.004 |

(b) Location 2:

| Gate | $C_d$ | $C_m$ | $C_{gd}$ | $C_g$ | $A=C_m/C_d$ | $B=1/(C_d/C_m+C_{gd}/C_g)$ | \|A-B\|/B |
|---|---|---|---|---|---|---|---|
| LEG | 2.17 | 0.35 | 0.420 | 6.83 | 0.161 | 0.160 | 0.006 |
| LCP | 2.17 | 0.35 | 0.031 | 1.69 | 0.161 | 0.161 | 0.000 |
| LLP | 2.17 | 0.35 | 0.024 | 0.66 | 0.161 | 0.160 | 0.006 |
| LIP | 2.17 | 0.35 | 0.071 | 0.53 | 0.161 | 0.158 | 0.019 |

(b) Location 3:

| Gate | $C_d$ | $C_m$ | $C_{gd}$ | $C_g$ | $A=C_m/C_d$ | $B=1/(C_d/C_m+C_{gd}/C_g)$ | \|A-B\|/B |
|---|---|---|---|---|---|---|---|
| LEG | 2.22 | 0.58 | 0.570 | 6.75 | 0.261 | 0.256 | 0.020 |
| LCP | 2.22 | 0.58 | 0.552 | 1.55 | 0.261 | 0.239 | 0.092* |
| LLP | 2.22 | 0.58 | 0.080 | 0.64 | 0.261 | 0.253 | 0.032 |
| LIP | 2.22 | 0.58 | 0.018 | 0.54 | 0.261 | 0.259 | 0.008 |

(b) Location 4:

| Gate | $C_d$ | $C_m$ | $C_{gd}$ | $C_g$ | $A=C_m/C_d$ | $B=1/(C_d/C_m+C_{gd}/C_g)$ | \|A-B\|/B |
|---|---|---|---|---|---|---|---|
| LEG | 2.31 | 0.29 | 0.288 | 6.86 | 0.126 | 0.125 | 0.005 |
| LCP | 2.31 | 0.29 | 1.094 | 1.56 | 0.126 | 0.115 | 0.088* |
| LLP | 2.31 | 0.29 | 0.097 | 0.65 | 0.126 | 0.123 | 0.019 |
| LIP | 2.31 | 0.29 | 0.02 | 0.54 | 0.126 | 0.125 | 0.005 |

Table S2. Capacitances (in aF) relevant to $Q_0(t)/\Delta Q_d$ when the defect is at different lateral locations but at the midpoint of the oxide thickness (z=-15 nm) while sweeping different gate voltages (LEG, LCP, LLP and LIP) for a "bare" device. $Q_0(t) \approx (C_m/C_d)\Delta Q_d$ for defects away from the gate. Data with * are for defects near the gate.

For "bare" and "TG" devices, Tables S2 and S3 show that for defects (z=-15 nm) away from the gate, $Q_0(t) \approx (C_m/C_d)\Delta Q_d$, independent of which gate is used in the measurement. We have also calculated these values when the defect is at z=-7 nm and z=-23 nm. All these results show that $Q_0(t) \approx (C_m/C_d)\Delta Q_d$ for defects away from the gate. For all calculated cases (with the defect away or near the gate), the maximum relative difference between the above

approximation ($A$) and the result ($B$) from Equation 4, $|A - B|/B$ is 12.3% (as shown in Table S3(a)). Therefore, we use $C_m/C_d$ to evaluate the charge offset drift reduction before and after adding the top gate. This also means that the charge offset drift can be measured independent of which gate is used to sweep the gate voltage.

(a) Location 1:

| Gate | $C_d$ | $C_m$ | $C_{gd}$ | $C_g$ | $A=C_m/C_d$ | $B=1/(C_d/C_m+C_{gd}/C_g)$ | $\|A-B\|/B$ |
|---|---|---|---|---|---|---|---|
| LEG | 2.64 | 1.26 | 1.22 | 4.74 | 0.477 | 0.425 | 0.123* |
| LCP | 2.64 | 1.26 | 0.002 | 0.74 | 0.477 | 0.477 | 0.001 |
| LLP | 2.64 | 1.26 | 0.0003 | 0.31 | 0.477 | 0.477 | 0.000 |
| LIP | 2.64 | 1.26 | 0.0003 | 0.24 | 0.477 | 0.477 | 0.001 |

(b) Location 2:

| Gate | $C_d$ | $C_m$ | $C_{gd}$ | $C_g$ | $A=C_m/C_d$ | $B=1/(C_d/C_m+C_{gd}/C_g)$ | $\|A-B\|/B$ |
|---|---|---|---|---|---|---|---|
| LEG | 2.53 | 0.15 | 0.025 | 5.27 | 0.059 | 0.059 | 0.000 |
| LCP | 2.53 | 0.15 | 0.006 | 0.74 | 0.059 | 0.059 | 0.000 |
| LLP | 2.53 | 0.15 | 0.006 | 0.31 | 0.059 | 0.059 | 0.001 |
| LIP | 2.53 | 0.15 | 0.014 | 0.26 | 0.059 | 0.059 | 0.003 |

(b) Location 3:

| Gate | $C_d$ | $C_m$ | $C_{gd}$ | $C_g$ | $A=C_m/C_d$ | $B=1/(C_d/C_m+C_{gd}/C_g)$ | $\|A-B\|/B$ |
|---|---|---|---|---|---|---|---|
| LEG | 2.54 | 0.35 | 0.08 | 5.26 | 0.138 | 0.138 | 0.002 |
| LCP | 2.54 | 0.35 | 0.126 | 0.72 | 0.138 | 0.135 | 0.024* |
| LLP | 2.54 | 0.35 | 0.017 | 0.31 | 0.138 | 0.137 | 0.008 |
| LIP | 2.54 | 0.35 | 0.005 | 0.24 | 0.138 | 0.137 | 0.003 |

(b) Location 4:

| Gate | $C_d$ | $C_m$ | $C_{gd}$ | $C_g$ | $A=C_m/C_d$ | $B=1/(C_d/C_m+C_{gd}/C_g)$ | $\|A-B\|/B$ |
|---|---|---|---|---|---|---|---|
| LEG | 2.46 | 0.16 | 0.024 | 5.27 | 0.065 | 0.065 | 0.000 |
| LCP | 2.46 | 0.16 | 0.73 | 0.69 | 0.065 | 0.061 | 0.069* |
| LLP | 2.46 | 0.16 | 0.029 | 0.31 | 0.065 | 0.065 | 0.006 |
| LIP | 2.46 | 0.16 | 0.007 | 0.24 | 0.065 | 0.065 | 0.002 |

Table S3. Capacitances (in aF) relevant to $Q_0(t)/\Delta Q_d$ when the defect is at different lateral locations (z=-15 nm) while sweeping different gate voltages (LEG, LCP, LLP and LIP) for a "TG" device. Data with * are for defects near the gate.

From Tables S4, S5 and S6, adding the top gate increases the total capacitance of charge defects and decreases the mutual capacitance to the quantum dot. Both effects can reduce the charge offset drift $Q_0(t)$. Along the z direction, near the $Si/SiO_2$ interface, the reduction is less effective (Table S5); at the middle of the oxide, the reduction is about a factor of two (Table S4); and near the $SiO_2$/gate interface, the reduction is larger than a factor of two (Table S6). Laterally, for defects located nearer the quantum dot or other gates, the reduction in $C_m/C_d$ due to the top gate is also more muted. The detailed spatial distribution of defects will impact the size of the change in $Q_0(t)$, however these calculations show that the observed reduction in $Q_0(t)$ can be accounted for by the electrostatic reduction in $C_m$ and increase in $C_d$, with the change in $C_m$ being dominant.

"bare": z=-15 nm

| Location | $C_d$ | $C_m$ | $A_{bare}=C_m/C_d$ |
|---|---|---|---|
| 1 | 2.64 | 1.29 | 0.49 |
| 2 | 2.17 | 0.35 | 0.16 |
| 3 | 2.22 | 0.58 | 0.26 |
| 4 | 2.31 | 0.29 | 0.13 |

"TG": z=-15 nm

| Location | $C_d$ | $C_m$ | $A_{TG}=C_m/C_d$ | $A_{bare}/A_{TG}$ |
|---|---|---|---|---|
| 1 | 2.64 | 1.26 | 0.48 | 1.02 |
| 2 | 2.53 | 0.15 | 0.06 | 2.67 |
| 3 | 2.54 | 0.35 | 0.13 | 2.0 |
| 4 | 2.46 | 0.16 | 0.07 | 1.86 |

Table S4. Capacitances (in aF) of the defect at different lateral locations (z=-15 nm) and the charge offset drift reduction with and without a top gate.

“bare”: z=-23 nm

| Location | $C_d$ | $C_m$ | $A_{bare}=C_m/C_d$ |
|---|---|---|---|
| 1 | 3.22 | 2.51 | 0.78 |
| 2 | 2.49 | 0.42 | 0.17 |
| 3 | 2.53 | 0.72 | 0.29 |
| 4 | 2.55 | 0.36 | 0.14 |

“TG”: z=-23 nm

| Location | $C_d$ | $C_m$ | $A_{TG}=C_m/C_d$ | $A_{bare}/A_{TG}$ |
|---|---|---|---|---|
| 1 | 3.17 | 2.44 | 0.77 | 1.0 |
| 2 | 2.65 | 0.24 | 0.09 | 1.9 |
| 3 | 2.65 | 0.54 | 0.20 | 1.4 |
| 4 | 2.62 | 0.25 | 0.10 | 1.5 |

Table S5. Capacitances (in aF) of the defect at different lateral locations (z=-23 nm) and the charge offset drift reduction with and without a top gate.

“bare”: z=-7 nm

| Location | $C_d$ | $C_m$ | $A_{bare}=C_m/C_d$ |
|---|---|---|---|
| 1 | 3.24 | 0.68 | 0.21 |
| 2 | 1.93 | 0.30 | 0.16 |
| 3 | 1.97 | 0.47 | 0.24 |
| 4 | 2.15 | 0.23 | 0.11 |

“TG”: z=-7 nm

| Location | $C_d$ | $C_m$ | $A_{TG}=C_m/C_d$ | $A_{bare}/A_{TG}$ |
|---|---|---|---|---|
| 1 | 3.22 | 0.65 | 0.20 | 1.0 |
| 2 | 3.19 | 0.08 | 0.025 | 6.2 |
| 3 | 3.21 | 0.20 | 0.062 | 3.8 |
| 4 | 2.58 | 0.10 | 0.039 | 2.8 |

Table S6. Capacitances (in aF) of the defect at different lateral locations with z=-7 nm and the charge offset drift reduction between “bare” and “TG” devices.

## S3: Charge offset drift data for device 5.4-23U and device 4.7-33U

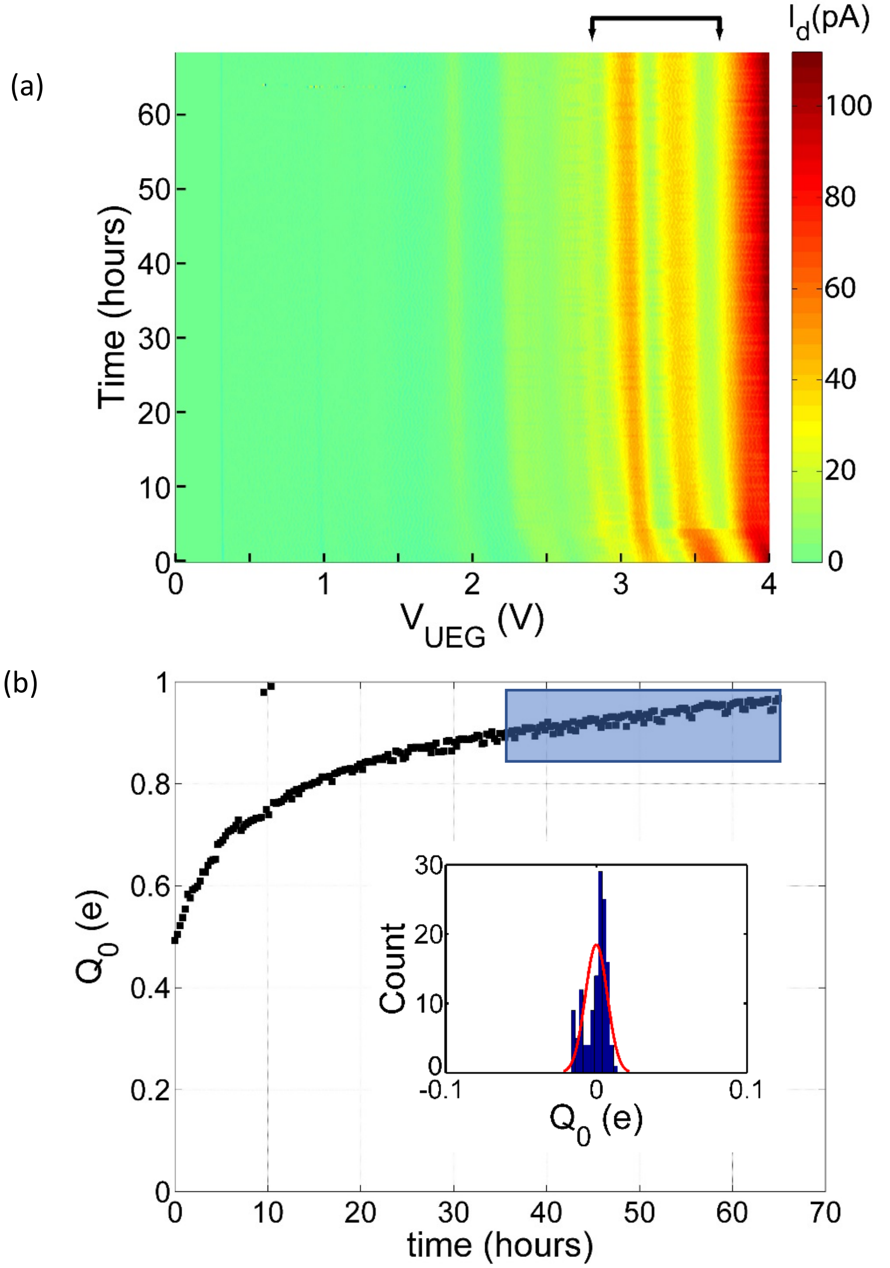


Figure S4. $Q_0(t)$ for a "TG" device (5.4-23U) using the NIST DC measurement system. (a) Data taken at $V_{TG}$ = 0.175V, $V_{d\_DC}$ = 3 mV and sweeping $V_{UEG}$ with other gates at 0V. (b) $Q_0$ extracted from the Coulomb blockade oscillations using a sinusoidal function in the range indicated by arrows as shown in (a). The shaded area shows a stable period, and the insets show the histogram of the fluctuation $\Delta Q_0$ after subtracting a linear-fit line with a standard deviation of 0.007 e (DC).

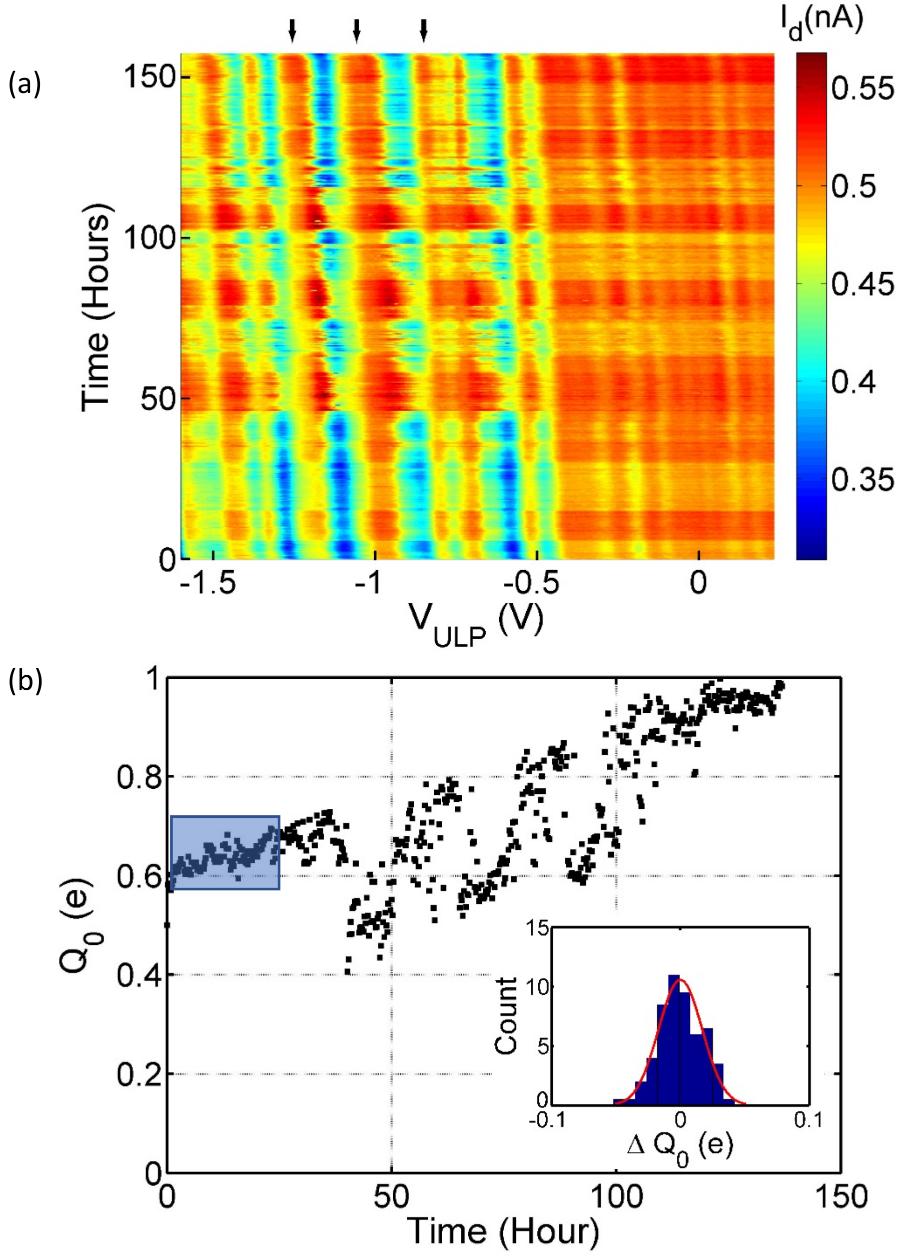


Figure S5. $Q_0(t)$ for a "bare" device (4.7-33U) using the CSUSM DC measurement system and cryostat. (a) Data taken at $V_{d\_DC}$=5 mV and sweeping $V_{ULP}$ with $V_{UEG}$=2.5 V, $V_{LIP}$=-0.8 V and other gates at 0 V. Extracted $Q_0(t)$ is shown in (b), using Gaussian functions with arrows indicating the three peaks used in the fitting. The shaded area shows a stable period, and the inset shows the histogram of the fluctuation $\Delta Q_0$ after subtracting a linear-fit line with a standard deviation of 0.017 e.
